# Supplementary material for: On the Limitations of Sociodemographic Adaptation with Transformers
Source: arXiv:2208.01029 source file (2022-08-01)
Supplement: Supplementary file 1 [file 99-appendix.tex]

\label{sec:appendix}
\onecolumn
\section{Additional Experiments.}

\setlength{\tabcolsep}{4.4pt}
\begin{table*}[htp!]
\centering
%\resizebox{\textwidth}{!}{%
\scriptsize{
\begin{tabular}{clcccccccccccccccc}
\toprule
\multicolumn{1}{l}{}              & \multicolumn{1}{c}{}         & \multicolumn{2}{c}{\textbf{AC-SA}} & \multicolumn{2}{c}{\textbf{AC-TD}} & \multicolumn{6}{c}{\textbf{SA}}                                             & \multicolumn{6}{c}{\textbf{TD}}                                             \\
\cmidrule(lr){3-4}\cmidrule(lr){5-6}\cmidrule(lr){7-12}\cmidrule(lr){13-18}
\multicolumn{1}{l}{}              &                              &                     &                     &                     &                     & \textbf{F} & \textbf{M} & \textbf{X} & \textbf{F} & \textbf{M} & \textbf{X} & \textbf{F} & \textbf{M} & \textbf{X} & \textbf{F} & \textbf{M} & \textbf{X} \\
\cmidrule(lr){7-9}\cmidrule(lr){10-12}\cmidrule(lr){13-15}\cmidrule(lr){16-18}
\multicolumn{1}{l}{\textit{\textbf{gender}}}              &       \textbf{Model}         & \textbf{Mono}       & \textbf{Multi}      & \textbf{Mono}       & \textbf{Multi}      & \multicolumn{3}{c}{\textbf{Mono}}    & \multicolumn{3}{c}{\textbf{Multi}}   & \multicolumn{3}{c}{\textbf{Mono}}    & \multicolumn{3}{c}{\textbf{Multi}}   \\
\midrule
\multirow{6}{*}{\textbf{Denmark}} & \textit{w/o specialization} & \multicolumn{1}{l}{} & \multicolumn{1}{l}{} & \multicolumn{1}{l}{} & \multicolumn{1}{l}{} & \multicolumn{1}{l}{} & \multicolumn{1}{l}{} & \multicolumn{1}{l}{} & \multicolumn{1}{l}{} & \multicolumn{1}{l}{} & \multicolumn{1}{l}{} & \multicolumn{1}{l}{} & \multicolumn{1}{l}{} & \multicolumn{1}{l}{} & \multicolumn{1}{l}{} & \multicolumn{1}{l}{} & \multicolumn{1}{l}{} \\
 & BERT & 66.1 & 64.0 & 63.8 & 61.8 & 72.3 & 67.9 & 70.4 & 69.2 & 64.8 & 67.2 & 60.7 & 59.8 & 59.9 & 59.3 & 58.3 & 59.0 \\\cmidrule(lr){2-18}
 & \textit{with specialization} &  &  &  &  &  &  &  & \multicolumn{1}{l}{} & \multicolumn{1}{l}{} & \multicolumn{1}{l}{} &  &  &  & \multicolumn{1}{l}{} & \multicolumn{1}{l}{} & \multicolumn{1}{l}{} \\
 & MLM & 66.0 & \textbf{65.2} & \textbf{64.2} & 63.4 & 72.5 & 68.3 & 70.3 & 69.5 & \textbf{65.8} & 67.8 & 60.6 & \textbf{60.6} & 60.6 & 59.7 & 58.8 & \textbf{59.4} \\
 & MTL-W (CLS) & \textbf{66.2} & 64.9 & 64.1 & 63.5 & \textbf{72.6} & \textbf{68.6} & \textbf{70.6} & \textbf{69.9} & 65.7 & 67.7 & \textbf{61.3} & 60.5 & 60.0 & 59.7 & 57.8 & 59.1 \\
 & MTL-W (CTX) & 66.0 & 65.0 & 64.1 & \textbf{63.5} & 72.4 & 68.4 & 70.6 & 69.1 & 65.6 & \textbf{68.0} & 61.1 & 60.2 & \textbf{60.8} & \textbf{59.9} & \textbf{58.9} & 59.0 \\\midrule
\multirow{6}{*}{\textbf{Germany}} & \textit{w/o specialization} &  &  &  &  &  &  &  &  &  &  &  &  &  &  &  &  \\
 & BERT & 59.8 & 59.5 & 58.9 & 57.9 & 66.5 & 63.7 & 64.3 & 66.1 & 63.2 & 64.5 & 67.9 & 66.1 & 67.8 & 67.8 & 65.6 & 65.8 \\\cmidrule(lr){2-18}
 & \textit{with specialization} &  &  &  &  &  &  &  & \multicolumn{1}{l}{} & \multicolumn{1}{l}{} & \multicolumn{1}{l}{} &  &  &  & \multicolumn{1}{l}{} & \multicolumn{1}{l}{} & \multicolumn{1}{l}{} \\
 & MLM & 62.0 & 61.2 & 59.7 & 60.1 & 68.1 & \textbf{65.8} & 65.4 & \textbf{67.7} & \textbf{65.3} & 66.1 & 68.5 & 66.7 & 67.7 & \textbf{68.6} & 67.0 & \textbf{67.1} \\
 & MTL-W (CLS) & \textbf{61.1} & 60.1 & 59.0 & \textbf{60.3} & \textbf{68.8} & 64.4 & \textbf{66.2} & 66.7 & 64.0 & 65.7 & \textbf{68.9} & 66.4 & 67.8 & 67.6 & 65.7 & 66.4 \\
 & MTL-W (CTX) & 60.9 & \textbf{62.9} & \textbf{60.3} & 58.3 & 67.9 & 65.6 & 66.0 & 66.8 & 64.3 & \textbf{66.8} & 68.6 & \textbf{66.8} & \textbf{67.9} & 68.3 & \textbf{67.0} & 66.7 \\\midrule
\multirow{6}{*}{\textbf{US}} & \textit{w/o specialization} &  &  &  &  &  &  &  &  &  &  &  &  &  &  &  &  \\
 & BERT & 64.3 & 62.6 & 58.7 & 58.1 & 68.6 & 67.0 & 67.1 & 66.3 & 64.4 & 66.0 & 72.5 & 69.7 & 71.0 & 71.2 & 68.4 & 70.2 \\\cmidrule(lr){2-18}
 & \textit{with specialization} &  &  &  &  &  &  &  &  &  &  &  &  &  &  &  &  \\
 & MLM & 64.6 & 63.3 & 58.7 & \textbf{59.6} & 68.4 & 67.6 & 67.8 & 67.3 & 66.2 & 66.9 & 73.1 & 70.1 & 71.3 & 72.1 & 69.4 & 70.3 \\
 & MTL-W (CLS) & 64.3 & \textbf{63.8} & 58.8 & 59.2 & 68.6 & \textbf{68.0} & \textbf{68.0} & 67.2 & 66.3 & 67.0 & 73.1 & \textbf{70.3} & 71.6 & 72.3 & 69.2 & 70.4 \\
 & MTL-W (CTX) & \textbf{64.7} & 62.2 & \textbf{59.4} & 58.8 & \textbf{68.9} & 67.5 & 67.9 & \textbf{68.0} & \textbf{66.4} & \textbf{67.3} & \textbf{73.3} & 69.9 & \textbf{71.6} & \textbf{72.8} & \textbf{69.5} & \textbf{70.5} \\\midrule
\multirow{6}{*}{\textbf{UK}} & \textit{w/o specialization} &  & \multicolumn{1}{l}{} &  &  &  &  &  &  &  &  &  &  &  &  &  &  \\
 & BERT & 63.2 & 61.9 & 65.0 & 63.1 & 73.4 & 71.0 & 72.3 & 71.0 & 69.0 & 69.7 & 71.2 & 69.1 & 70.1 & 70.4 & 67.9 & 68.9 \\\cmidrule(lr){2-18}
 & \textit{with specialization} &  &  &  &  &  &  &  &  &  &  &  &  &  &  &  &  \\
 & MLM & \textbf{63.7} & 63.0 & 64.8 & 65.3 & \textbf{73.9} & 71.0 & \textbf{72.6} & 72.0 & 70.4 & 71.0 & 71.2 & \textbf{69.4} & 70.0 & 70.6 & 67.9 & 69.8 \\
 & MTL-W (CLS) & 63.2 & 63.4 & \textbf{65.2} & 64.9 & 73.6 & \textbf{72.2} & 72.4 & 72.9 & 70.9 & 71.7 & \textbf{71.5} & 69.3 & 70.2 & 70.6 & 68.2 & 69.8 \\
 & MTL-W (CTX) & 63.3 & \textbf{63.5} & 64.8 & \textbf{65.6} & 73.7 & 72.0 & 72.2 & \textbf{73.0} & \textbf{71.0} & \textbf{71.9} & 71.4 & 69.1 & \textbf{70.3} & \textbf{70.8} & \textbf{68.2} & \textbf{69.9} \\\midrule
\multirow{6}{*}{\textbf{France}} & \textit{w/o specialization} &  &  &  &  &  &  &  &  &  &  &  &  &  &  &  &  \\
 & BERT & 64.1 & 63.9 & 63.1 & 61.2 & 70.5 & 67.3 & 68.6 & 69.3 & 67.0 & 67.8 & 46.0 & \textbf{44.5} & 45.1 & 44.6 & 42.4 & 43.1 \\\cmidrule(lr){2-18}
 & \textit{with specialization} &  &  &  &  &  &  &  &  &  &  &  &  &  &  &  &  \\
 & MLM & \textbf{64.9} & 64.6 & \textbf{63.2} & 62.1 & 71.0 & 67.7 & 67.6 & 69.9 & 67.1 & 68.4 & 46.2 & 44.3 & 45.5 & 45.8 & 43.3 & 44.3 \\
 & MTL-W (CLS) & 64.2 & 64.1 & 63.1 & \textbf{63.1} & 70.5 & 67.5 & 69.3 & \textbf{70.6} & 67.3 & 68.4 & \textbf{47.1} & 44.2 & 45.3 & \textbf{46.0} & 43.4 & 44.2 \\
 & MTL-W (CTX) & 64.4 & \textbf{65.0} & 62.9 & 62.9 & \textbf{71.7} & \textbf{68.3} & \textbf{69.5} & 70.1 & \textbf{67.5} & \textbf{68.8} & 46.9 & 44.3 & \textbf{45.6} & 45.5 & \textbf{43.9} & \textbf{44.4}\\\bottomrule
\end{tabular}%
}
\vspace{-0.3em}
\caption{Evaluation results compared with monolingual BERT and multilingual BERT (mBERT) on five countries with \textit{gender} data for three tasks: attribute classification (AC-SA, AC-TD), sentiment analysis (SA) and topic detection (TD).}
\label{tab:mono_multi_compare_gender}
\end{table*}

\setlength{\tabcolsep}{4.4pt}
\begin{table*}[t]
\centering
\vspace{-0.3em}
%\sisetup{round-mode=places,round-precision=1, detect-all,detect-weight=true, detect-family=true}
%\resizebox{\textwidth}{!}{%
\scriptsize{
\begin{tabular}{clcccccccccccccccc}
\toprule
\multicolumn{1}{l}{}              & \multicolumn{1}{c}{}         & \multicolumn{2}{c}{\textbf{AC-SA}} & \multicolumn{2}{c}{\textbf{AC-TD}} & \multicolumn{6}{c}{\textbf{SA}}                                             & \multicolumn{6}{c}{\textbf{TD}}                                             \\
\cmidrule(lr){3-4}\cmidrule(lr){5-6}\cmidrule(lr){7-12}\cmidrule(lr){13-18}
\multicolumn{1}{l}{}              &                              &                     &                     &                     &                     & \textbf{0} & \textbf{2} & \textbf{X} & \textbf{0} & \textbf{2} & \textbf{X} & \textbf{0} & \textbf{2} & \textbf{X} & \textbf{0} & \textbf{2} & \textbf{X} \\
\cmidrule(lr){7-9}\cmidrule(lr){10-12}\cmidrule(lr){13-15}\cmidrule(lr){16-18}
\multicolumn{1}{l}{\textit{\textbf{age}}}              &       \textbf{Model}         & \textbf{Mono}       & \textbf{Multi}      & \textbf{Mono}       & \textbf{Multi}      & \multicolumn{3}{c}{\textbf{Mono}}    & \multicolumn{3}{c}{\textbf{Multi}}   & \multicolumn{3}{c}{\textbf{Mono}}    & \multicolumn{3}{c}{\textbf{Multi}}   \\
\midrule
\multirow{6}{*}{\textbf{Denmark}} & \textit{w/o specialization} &  & \multicolumn{1}{l}{} & \multicolumn{1}{l}{} & \multicolumn{1}{l}{} & \multicolumn{1}{l}{} & \multicolumn{1}{l}{} & \multicolumn{1}{l}{} & \multicolumn{1}{l}{} & \multicolumn{1}{l}{} & \multicolumn{1}{l}{} & \multicolumn{1}{l}{} & \multicolumn{1}{l}{} & \multicolumn{1}{l}{} & \multicolumn{1}{l}{} & \multicolumn{1}{l}{} & \multicolumn{1}{l}{} \\
 & BERT & 67.7 & 57.2 & 65.3 & 64.5 & 67.3 & 66.2 & 66.0 & 62.7 & 62.7 & 62.9 & 58.4 & 54.4 & 56.3 & 56.1 & 52.2 & 53.4 \\\cmidrule(lr){2-18}
 & \textit{with specialization} &  &  &  &  &  &  &  &  &  &  &  &  &  &  &  &  \\
 & MLM & 67.4 & \textbf{65.5} & \textbf{67.4} & 65.1 & \textbf{67.7} & \textbf{67.3} & \textbf{67.6} & 63.3 & 62.1 & 63.0 & \textbf{59.3} & 55.3 & \textbf{57.6} & \textbf{57.1} & 52.6 & 54.1 \\
 & MTL-W (CLS) & 67.4 & 65.2 & 66.8 & \textbf{65.2} & 67.4 & 66.2 & 67.1 & 63.1 & 62.9 & 63.0 & 58.7 & 55.0 & 56.5 & 56.9 & \textbf{53.3} & \textbf{54.5} \\
 & MTL-W (CTX) & \textbf{67.8} & 65.3 & 66.6 & 64.6 & 67.6 & 66.1 & 67.2 & \textbf{64.2} & \textbf{63.3} & \textbf{63.2} & 59.0 & \textbf{55.4} & 56.7 & 56.2 & 53.2 & 54.3 \\\midrule
\multirow{6}{*}{\textbf{Germany}} & \textit{w/o specialization} &  &  &  &  &  &  &  &  &  &  &  &  &  &  &  &  \\
 & BERT & 57.9 & 58.0 & 59.6 & 56.9 & 53.6 & 57.9 & 57.1 & 52.6 & 55.0 & 55.0 & 61.6 & 57.4 & 58.3 & 60.1 & 55.3 & 57.1 \\\cmidrule(lr){2-18}
 & \textit{with specialization} &  &  &  &  &  &  &  &  &  &  &  &  &  &  &  &  \\
 & MLM & 58.1 & \textbf{61.1} & \textbf{62.0} & \textbf{58.9} & \textbf{58.1} & \textbf{58.2} & \textbf{58.1} & 53.6 & 55.5 & 56.7 & 62.2 & 57.6 & \textbf{59.9} & \textbf{61.5} & 56.5 & 58.7 \\
 & MTL-W (CLS) & \textbf{58.2} & 56.4 & 61.3 & 58.2 & 56.3 & 57.3 & 55.8 & \textbf{53.8} & 55.3 & 55.5 & 63.5 & 57.9 & 59.1 & 60.8 & \textbf{57.6} & \textbf{59.3} \\
 & MTL-W (CTX) & 57.2 & 56.6 & 60.6 & 57.4 & 57.9 & 58.1 & 54.0 & 53.0 & \textbf{56.5} & \textbf{56.7} & \textbf{63.5} & \textbf{58.2} & 59.2 & 59.3 & 56.5 & 59.3 \\\midrule
\multirow{6}{*}{\textbf{US}} & \textit{w/o specialization} &  &  &  &  &  &  &  &  &  &  &  &  &  &  &  &  \\
 & BERT & 65.2 & 62.9 & 63.0 & 60.7 & 60.5 & 58.7 & 57.2 & 57.7 & 57.9 & 57.8 & 68.8 & 64.9 & \textbf{67.2} & 68.0 & 64.3 & 64.3 \\\cmidrule(lr){2-18}
 & \textit{with specialization} &  &  &  &  &  &  &  &  &  &  &  &  &  &  &  &  \\
 & MLM & 65.3 & \textbf{63.6} & 62.9 & \textbf{61.9} & 59.8 & \textbf{59.5} & \textbf{60.4} & 59.4 & 57.8 & \textbf{58.2} & 71.2 & 65.7 & 66.7 & 69.0 & 64.2 & 65.2 \\
 & MTL-W (CLS) & \textbf{66.2} & 60.7 & \textbf{64.1} & 61.5 & \textbf{61.6} & 58.3 & 59.4 & 59.3 & 57.9 & 58.0 & \textbf{72.5} & 65.5 & 67.1 & \textbf{69.8} & 64.4 & \textbf{65.8} \\
 & MTL-W (CTX) & 65.7 & 59.7 & 62.9 & 61.2 & 61.1 & 58.7 & 59.4 & \textbf{59.9} & \textbf{58.6} & 57.8 & 69.4 & \textbf{65.7} & 66.7 & 69.2 & \textbf{65.4} & 64.9 \\\midrule
\multirow{6}{*}{\textbf{UK}} & \textit{w/o specialization} &  &  &  &  &  &  &  &  &  &  &  &  &  &  &  &  \\
 & BERT & 65.7 & 65.1 & 65.8 & 65.2 & 65.2 & 66.3 & 65.5 & 63.8 & 63.9 & 63.7 & 68.1 & 68.1 & 68.0 & 64.7 & 67.1 & 66.3 \\\cmidrule(lr){2-18}
 & \textit{with specialization} &  &  &  &  &  &  &  &  &  &  &  &  &  &  &  &  \\
 & MLM & 66.9 & \textbf{65.4} & \textbf{66.1} & \textbf{65.6} & \textbf{68.2} & \textbf{67.2} & 66.9 & 62.8 & 62.0 & 63.0 & \textbf{68.8} & \textbf{70.1} & \textbf{70.0} & 65.1 & 67.3 & 67.3 \\
 & MTL-W (CLS) & 67.0 & 65.3 & 64.7 & 62.8 & 67.8 & 66.4 & \textbf{67.6} & 63.8 & 64.9 & 64.9 & 67.8 & 68.9 & 69.4 & 66.0 & \textbf{68.1} & 66.5 \\
 & MTL-W (CTX) & \textbf{66.8} & 64.0 & 65.2 & 62.8 & 67.6 & 66.5 & 67.1 & \textbf{64.6} & \textbf{65.2} & \textbf{65.1} & 68.2 & 69.6 & 69.2 & \textbf{66.4} & 67.3 & \textbf{67.6} \\\midrule
\multirow{6}{*}{\textbf{France}} & \textit{w/o specialization} &  &  &  &  &  &  &  &  &  &  &  &  &  &  &  &  \\
 & BERT & \textbf{56.0} & 55.7 & \textbf{57.0} & 56.6 & 59.7 & 57.5 & 60.3 & 59.6 & 57.4 & 61.5 & 51.9 & 49.1 & 49.6 & 52.0 & 47.1 & 49.0 \\\cmidrule(lr){2-18}
 & \textit{with specialization} &  &  &  &  &  &  &  &  &  &  &  &  &  &  &  &  \\
 & MLM & 55.9 & \textbf{56.8} & 56.9 & \textbf{57.2} & 60.7 & 59.4 & 61.6 & 59.9 & 59.5 & 61.6 & 53.8 & 48.5 & 50.2 & \textbf{52.5} & 47.2 & 50.3 \\
 & MTL-W (CLS) & 55.5 & 55.1 & 56.7 & 55.5 & \textbf{61.3} & 58.7 & \textbf{62.0} & 60.4 & \textbf{60.3} & \textbf{62.8} & 53.8 & 49.0 & 50.2 & 51.1 & 47.3 & 50.3 \\
 & MTL-W (CTX) & 55.8 & 54.4 & 56.7 & 55.9 & 60.2 & \textbf{60.7} & 61.5 & \textbf{60.9} & 59.8 & 59.7 & \textbf{54.6} & \textbf{51.4} & \textbf{50.3} & 50.2 & \textbf{48.0} & \textbf{50.8}
 \\
                                  \bottomrule
\end{tabular}%
}
\vspace{-0.3em}
\caption{Evaluation results compared with monolingual BERT and multilingual BERT (mBERT) on five countries with \textit{age} data for three tasks: attribute classification (AC-SA, AC-TD), sentiment analysis (SA) and topic detection (TD).}
\label{tab:mono_multi_compare_age}
\end{table*}

\setlength{\tabcolsep}{6.6pt}
\begin{table*}[t]
\centering
\footnotesize{%
\begin{tabular}{llcccccccccccc}
\toprule
% \multicolumn{14}{l}{} \\
 \textit{\textbf{gender}}&  & \multicolumn{6}{c}{\textbf{SA}} & \multicolumn{6}{c}{\textbf{TD}} \\\cmidrule(lr){3-8}\cmidrule(lr){9-14}
 &  & \textbf{F} & \textbf{M} & \textbf{X} & \textbf{F} & \textbf{M} & \textbf{X} & \textbf{F} & \textbf{M} & \textbf{X} & \textbf{F} & \textbf{M} & \textbf{X} \\\cmidrule(lr){3-5}\cmidrule(lr){6-8}\cmidrule(lr){9-11}\cmidrule(lr){12-14}
 & \textbf{Model} & \multicolumn{3}{c}{\textbf{RtGender}} & \multicolumn{3}{c}{\textbf{Trustpilot}} & \multicolumn{3}{c}{\textbf{RtGender}} & \multicolumn{3}{c}{\textbf{Trustpilot}} \\\midrule
\multirow{3}{*}{\textbf{US}} & MLM & 68.3 & 67.3 & 66.9 & 68.4 & 67.6 & 67.8 & \textbf{72.7} & \textbf{69.9} & 71.1 & 73.1 & 70.1 & 71.3 \\
 & MTL-W (CLS) & 68.1 & \textbf{67.4} & \textbf{66.9} & 68.6 & \textbf{68.0} & \textbf{68.0} & 72.7 & 69.3 & \textbf{71.2} & 73.1 & \textbf{70.3} & 71.6 \\
 & MTL-W (CTX) & \textbf{68.6} & 67.2 & 66.4 & \textbf{68.9} & 67.5 & 67.9 & 72.4 & 69.6 & 71.2 & \textbf{73.3} & 69.9 & \textbf{71.6} \\\midrule
\multirow{3}{*}{\textbf{UK}} & MLM & 73.3 & 71.0 & 71.7 & \textbf{73.9} & 71.0 & \textbf{72.6} & 71.1 & \textbf{69.3} & \textbf{69.8} & 71.2 & \textbf{69.4} & 70.0 \\
 & MTL-W (CLS) & 73.3 & 71.1 & \textbf{71.9} & 73.6 & \textbf{72.2} & 72.4 & 71.2 & 69.0 & 69.5 & \textbf{71.5} & 69.3 & 70.2 \\
 & MTL-W (CTX) & \textbf{73.4} & \textbf{71.1} & 71.6 & 73.7 & 72.0 & 72.2 & \textbf{71.3} & 69.2 & 69.6 & 71.4 & 69.1 & \textbf{70.3} \\\midrule\midrule
%\multicolumn{14}{l}{\textit{\textbf{age}}} \\
\textit{\textbf{age}} & \multicolumn{1}{c}{} & \multicolumn{6}{c}{\textbf{SA}} & \multicolumn{6}{c}{\textbf{TD}} \\\cmidrule(lr){3-8}\cmidrule(lr){9-14}
\multicolumn{1}{c}{} & \multicolumn{1}{c}{} & \textbf{0} & \textbf{2} & \textbf{X} & \textbf{0} & \textbf{2} & \textbf{X} & \textbf{0} & \textbf{2} & \textbf{X} & \textbf{0} & \textbf{2} & \textbf{X} \\\cmidrule(lr){3-5}\cmidrule(lr){6-8}\cmidrule(lr){9-11}\cmidrule(lr){12-14}
\multicolumn{1}{c}{} & \multicolumn{1}{c}{} & \multicolumn{3}{c}{\textbf{BAC}} & \multicolumn{3}{c}{\textbf{Trustpilot}} & \multicolumn{3}{c}{\textbf{BAC}} & \multicolumn{3}{c}{\textbf{Trustpilot}} \\\midrule
\multirow{3}{*}{\textbf{US}} & MLM & \textbf{59.4} & 58.4 & \textbf{58.9} & 59.8 & \textbf{59.5} & \textbf{60.4} & 68.4 & 64.6 & 66.9 & 71.2 & 65.7 & 66.7 \\
 & MTL-W (CLS) & 58.4 & 57.3 & 58.0 & \textbf{61.6} & 58.3 & 59.4 & 68.6 & 64.5 & \textbf{67.3} & \textbf{72.5} & 65.5 & \textbf{67.1} \\
 & MTL-W (CTX) & 58.6 & \textbf{58.5} & 58.9 & 61.1 & 58.7 & 59.4 & \textbf{69.3} & \textbf{65.0} & 67.1 & 69.4 & \textbf{65.7} & 66.7 \\\midrule
\multirow{3}{*}{\textbf{UK}} & MLM & 66.2 & \textbf{66.7} & 66.4 & \textbf{68.2} & \textbf{67.2} & 66.9 & 67.8 & 68.7 & 68.9 & \textbf{68.8} & \textbf{70.1} & \textbf{70.0} \\
 & MTL-W (CLS) & 66.1 & 66.6 & \textbf{66.8} & 67.8 & 66.4 & \textbf{67.6} & 67.8 & 68.7 & 68.6 & 67.8 & 68.9 & 69.4 \\
 & MTL-W (CTX) & \textbf{66.6} & 66.0 & 66.3 & 67.6 & 66.5 & 67.1 & \textbf{68.0} & \textbf{68.8} & \textbf{69.2} & 68.2 & 69.6 & 69.2 \\
 \bottomrule
\end{tabular}%
}
\caption{Evaluation results on trustpilot classification tasks compared by specializing on out-domain data (RtGender~\citep{voigt-etal-2018-rtgender} for \textit{gender} and BAC~\citep{schler2006effects} for \textit{age}) and in-domain data (Trustpilot).}
\label{tab:domain_compare}
\end{table*}
